# Supplementary material for: A unifying framework for generalised Bayesian online learning in non-stationary environments
Source: arXiv:2411.10153 source file (2025-03-12)
Supplement: Supplementary file 1 [file additional-experiments.tex]

\section{Additional experiments}
\label{sec:experiments-additional}

\subsection{Non-stationary heavy-tailed linear regression}
\label{experiment:heavy-tail-regression}

In this experiment,
we show  the flexibility of the framework and we derive a new method for online learning in the presence of outliers.

The true DGP consists of a
 piecewise linear regression model with Student-$t$ errors,
where the measurement are sampled according to
$\vx_t \sim {\cal U}[-2, 2]$,
$ \vy_t \sim {\rm St}\big( \phi(\vx_t)^\intercal\vtheta_t, 1,\,\, 2.01 \big)$
a Student-$t$ distribution with location $ \phi(\vx_t)^\intercal\vtheta_t$,
scale $1$ and degrees of freedom $2.01$, and
% \begin{equation}
% \begin{aligned}
%     \vx_t &\sim {\cal U}[-2, 2], &
%     \vy_t &\sim {\rm St}\big(
%     \underbrace{\phi(\vx_t)^\intercal\vtheta_t}_{\text{location}}, \underbrace{1,\,\, 2.01}_{\text{scale \& d.o.f.}}
%     \big),
% \end{aligned}
% \end{equation}
$\phi(\vx_t) = (1,\,x,\,x^2)$.
At every timestep, the parameters take the value
\begin{equation}
\vtheta_t =
\begin{cases}
\vtheta_{t-1} & \text{w.p. } 1 - p_\epsilon,\\
{\cal U}[-3, 3]^3 & \text{w.p. } p_\epsilon,
\end{cases}
\end{equation}
with $p_\epsilon = 0.001$, and $\vtheta_0 \sim {\cal U}[-3, 3]^3$. 
Intuitively, at each timestep, there is probability $p_\epsilon$  of a changepoint, and conditional on a changepoint occurring, the each of the entries of the new parameters $\vtheta_t$ are sampled from a uniform in $[-3,3]$. 
Figure \ref{fig:segements-tdlist-lr} shows some sample data generated by  this process.

\begin{figure}[htb]
    \centering
    \includegraphics[width=0.8\linewidth]{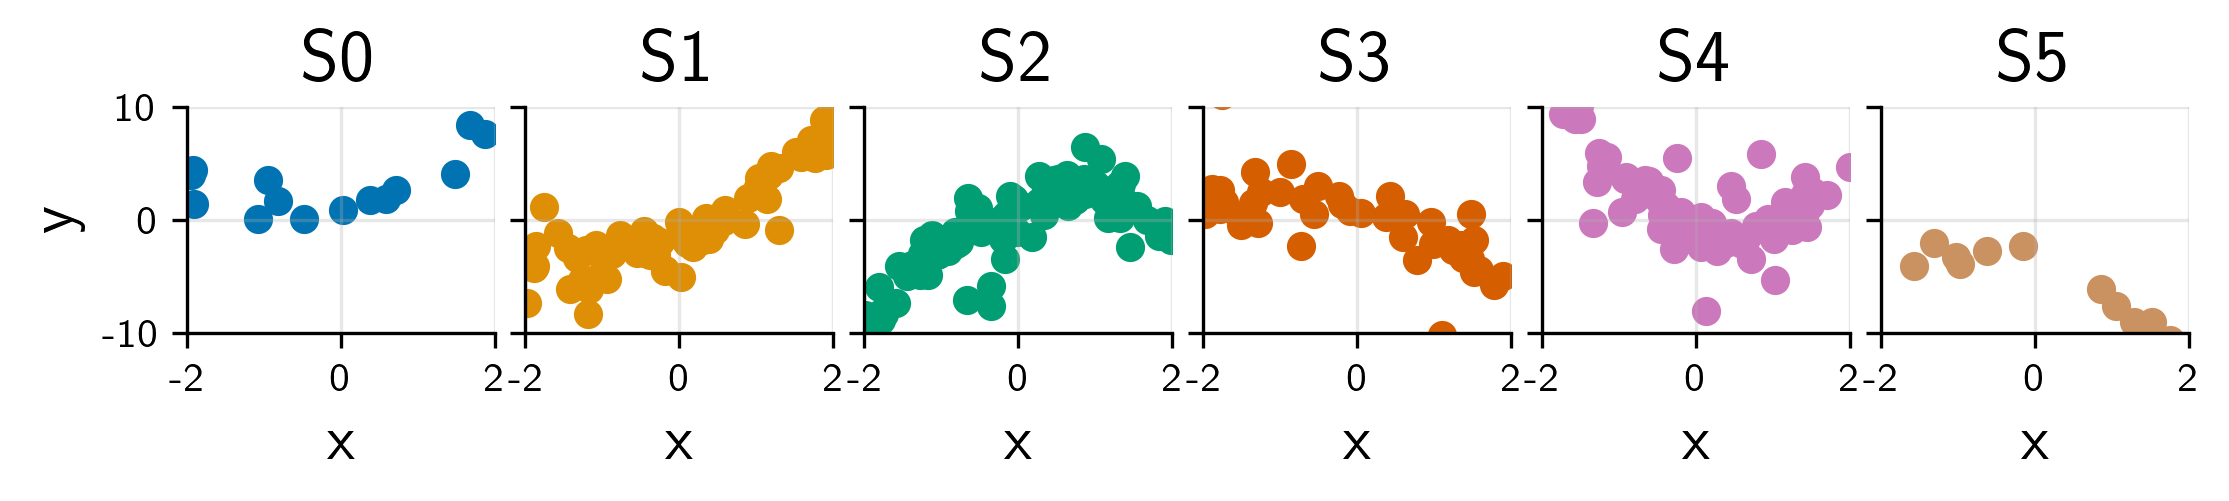}
    \vspace{-2em}
    \caption{
        Sample run of the heavy-tailed-regression process.
        Each box corresponds to the samples within a segment.
    }
    \label{fig:segements-tdlist-lr}
\end{figure}

Now we discuss how to fit this data.
For the measurement model \cModel,
we pick $h(\vtheta_t, \vx_t) = \vtheta_t^\intercal\,\vx_t$.
For the
auxiliary variable \cAux we choose
the runlength $\auxv_t = r_t$.
For the 
conditional prior \cPrior we use
the prior reset in
\eqref{eq:cprior-rl-pr}.
%This combination is known as \RLPR and it was introduced in \cite{adams2007bocd}. 
We work with the full memory version of the hypotheses for the trajectory of the runlength.

It is well-known that \RLPR is sensitive to outliers if the choice of \cModel is misspecified \citep{altamirano2023robust},
since an observation that is ``unusual'' may trigger a changepoint unnecessarily.
As a consequence,
many methods have proposed outlier-robust variants to the \RLPR for segmentation in the presence of outliers
(see e.g., \cite{fearnhead2019robustchangepoint, altamirano2023robust}).
In this experiment, however, we show that an outlier-robust variant of \RLPR for prediction can be created from the
filtering literature by changing the posterior  \cPosterior.
Specifically, because the choice of \cPosterior does not depend on \cPrior or \cAux,
we can make use of the vast literature for outlier-robust filtering in measurement space
\citep[see e.g.,][]{ting2007learning, agamennoni2012, piche2012, huang2016, wang2018}
to construct a robust and adaptive online learner by fixing \cAux and \cPrior to be \RLPR and changing \cPosterior.
In what follows, we consider the WoLF-IMQ method of \cite{duranmartin2024-wlf}
with soft threshold value set to three (representing three standard deviations). We use  WoLF-IMQ 
because it is a provably robust algorithm and it is a 
straightforward modification of the \texttt{LG} choice of \cPosterior.
We denote
the \RLPR with \cPosterior taken to be LG as \RLPRKF and
the \RLPR with \cPosterior taken to be WoLF-IMQ as \RLPRWoLF.
For this experiment, we consider the full set of hypotheses for each \texttt{RL} method,
i.e., the total number of computations increases at a linear rate in time,
as specified in Table \ref{tab:auxv-time-complexity}.

%\paragraph{Results}
The left panel in Figure \ref{fig:outliers-lr-res} shows
the rolling mean (with a window of size 10) of the RMSE for
\RLPRKF, \RLPRWoLF, and \staticKF.
Here, \staticKF corresponds to Bayesian update over a linear model without
any assumption of stationarity.
% Here, \staticKF is a baseline that assumes stationarity; in the nomenclature of our framework, \staticKF uses \texttt{C} as \cAux, \texttt{ACI} with $\gamma_t = 0$ for \cPrior, and \texttt{KF} for \cPosterior.
In this run, only a single changepoint occurs.
The right panel in Figure \ref{fig:outliers-lr-res}
shows the distribution of the RMSE for all methods after 30 trials.
\begin{figure}[htb]
    \centering
    \includegraphics[width=0.48\linewidth]{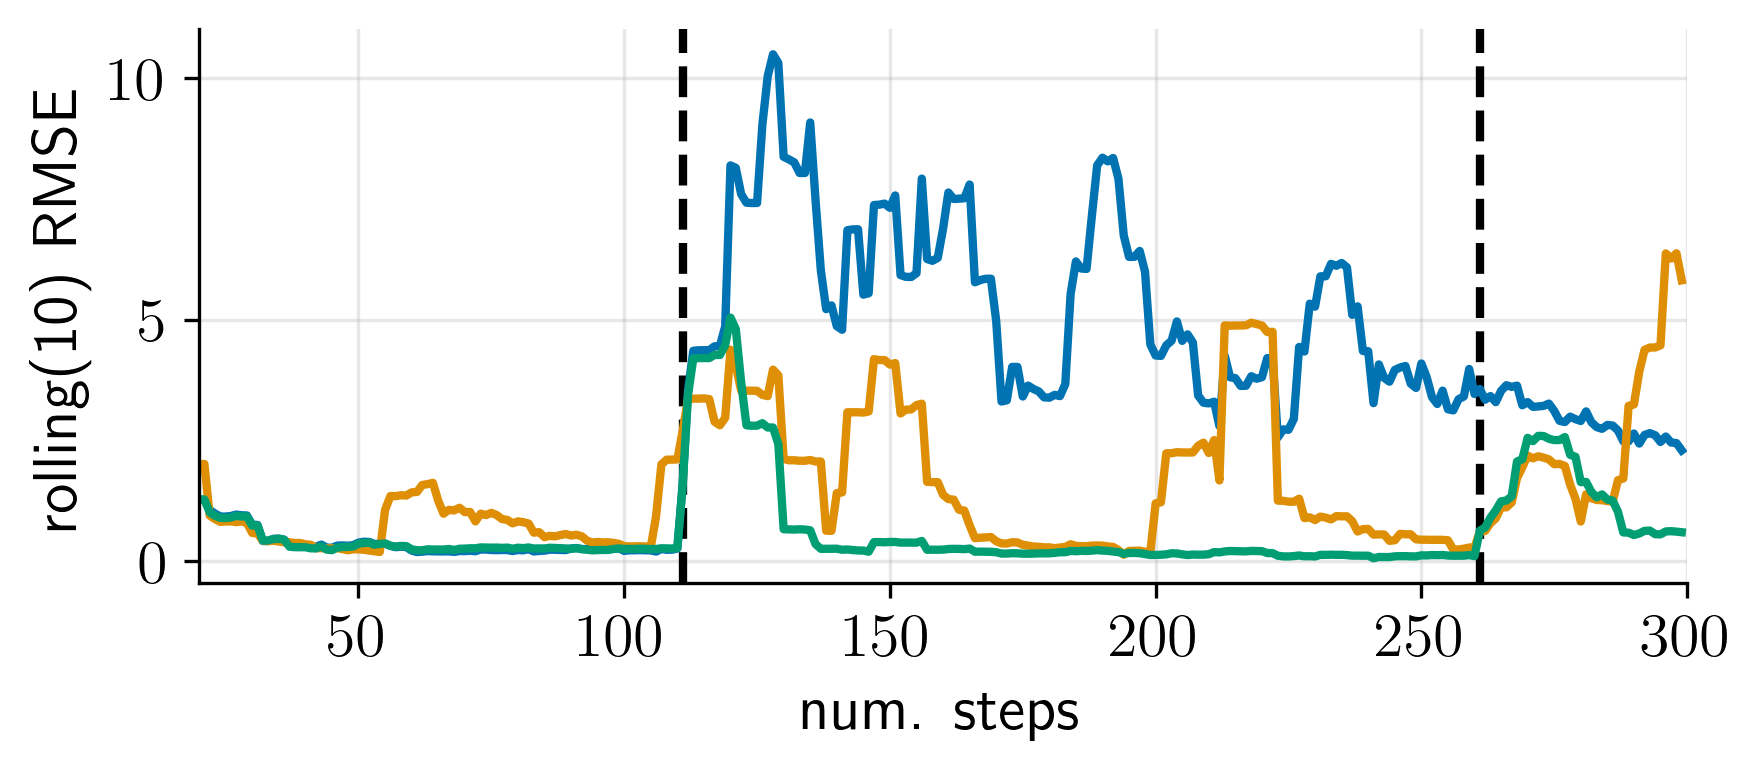}
    \includegraphics[width=0.48\linewidth]{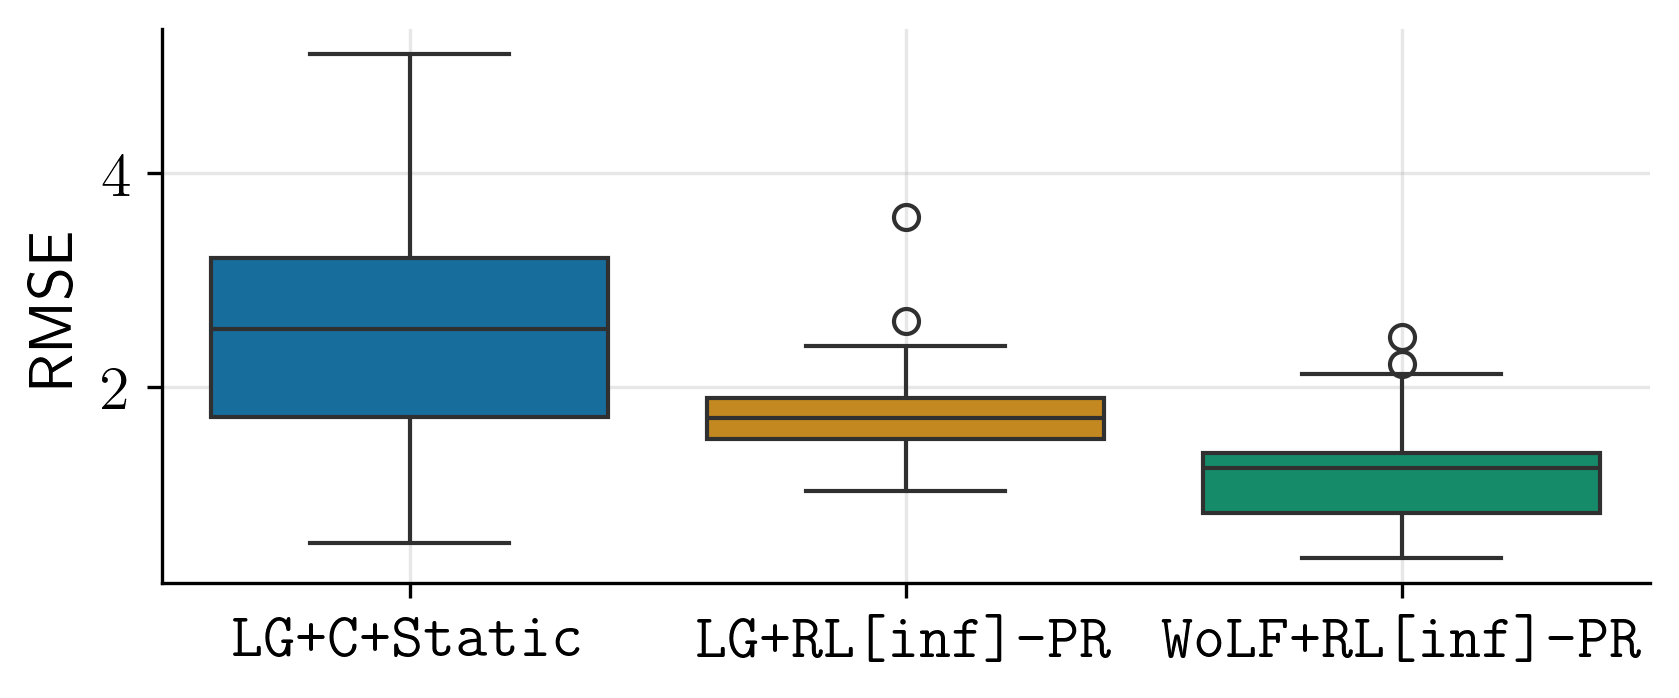}
    \caption{
    The \textbf{left panel} shows the rolling RMSE using a window of the 10 previous observations.
    The \textbf{right panel} shows the distribution of final RMSE over 30 runs.
    The vertical dotted line denotes a change in the true model parameters.
    }
    \label{fig:outliers-lr-res}
\end{figure}
We observe that \staticKF has much lower rolling RMSE error than \RLPRKF until the first regime change.
Its performance significantly deteriorates afterwards.
Next, \RLPRKF wrongly detects changepoints and resets its parameters frequently.
This results in periods of increased rolling RMSE.
Finally, \RLPRWoLF has the lowest error among the methods.
After the regime change, its error increases at a similar rate to the \staticKF,
however, it correctly adapts to the regime and its error decreases after around fifty steps.

Figure \ref{fig:bocd-lr-stress} shows
the log posterior estimate of the value of the runlength  after a single run
using \RLPRKF and \RLPRWoLF. In this plot we use $p_\epsilon = 0.01$  so that the changepoints are more frequent.
\begin{figure}[htb]
    \centering
    \includegraphics[width=0.48\linewidth]{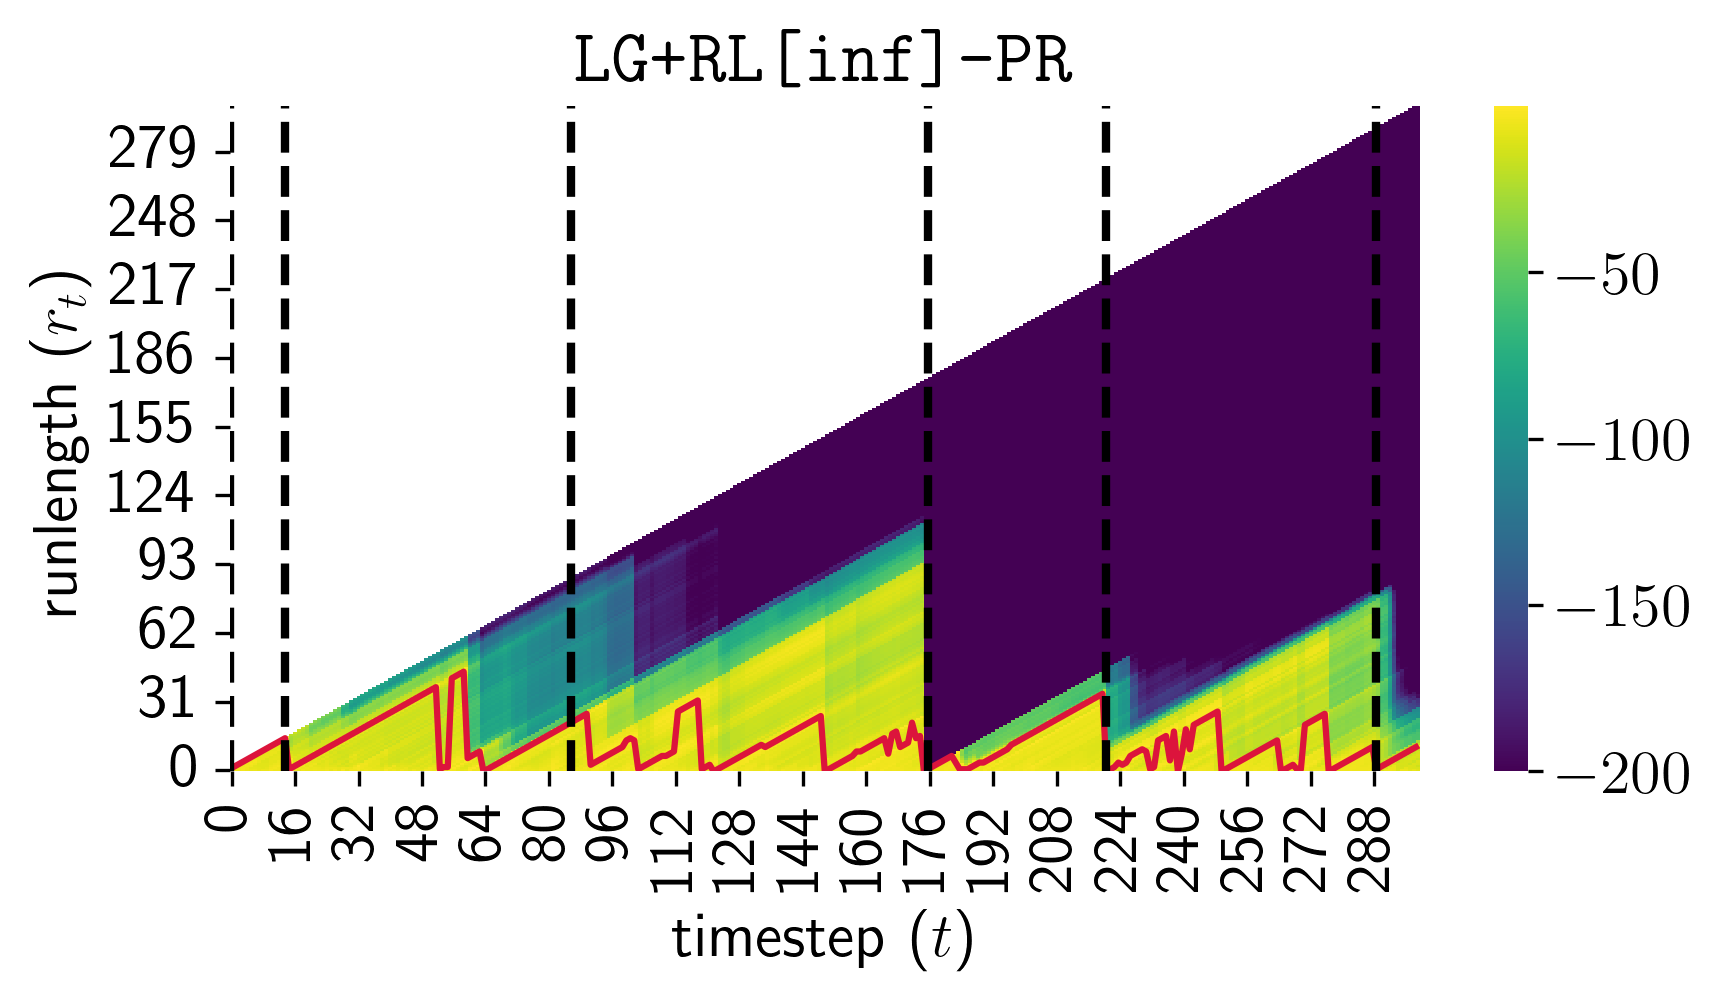}
    \includegraphics[width=0.48\linewidth]{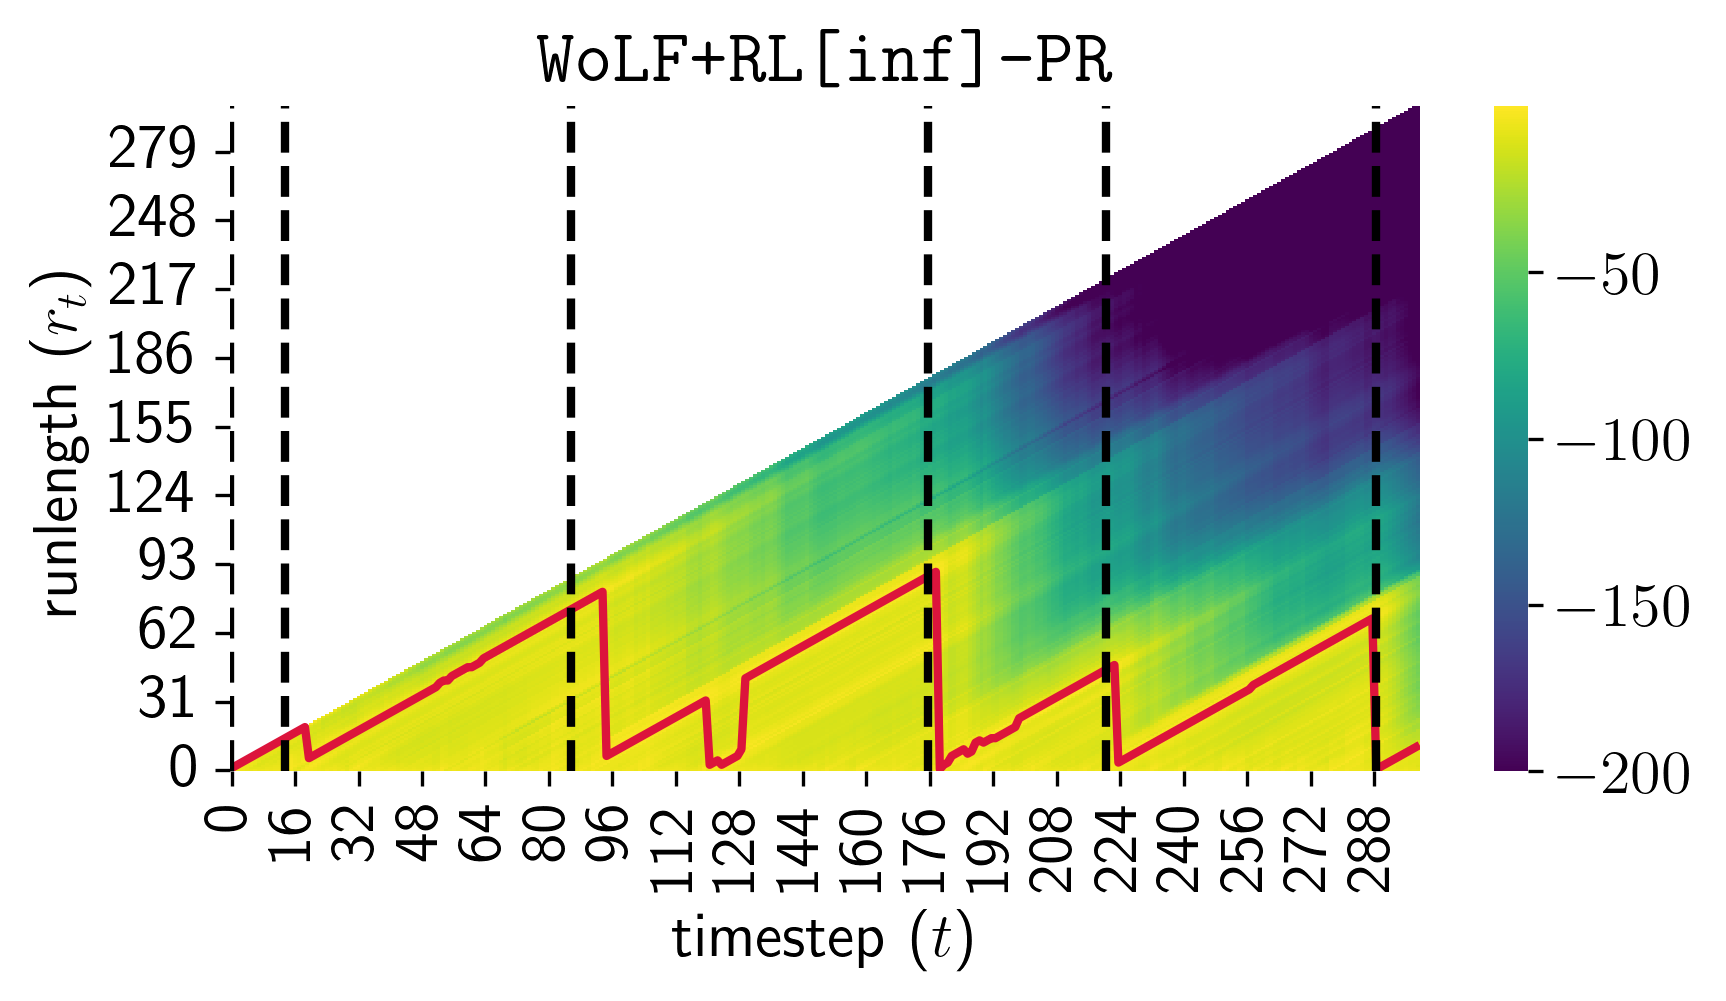}
    \caption{
        Segmentation of the non-stationary linear regression problem.
        The left panel shows the segmentation done by \RLPRKF.
        The right panel shows the segmentation done by \RLPRWoLF.
        The $x$-axis is the timestep $t$, the $y$-axis is the runlength $r_t$ (note that it is always the case that $r_t\leq t$), and the colour bar shows the value $\log\,p(r_t \cond \vy_{1:t})$.
        The red line in either plot is the trajectory of the mode, i.e.,
        the set $r_{1:t}^* = \{\argmax_{r_{1}} p(r_1 \cond \data_{1}),  \ldots, \argmax_{r_{t}} p(r_t \cond \data_{1:t})\}$. The dotted vertical lines are the  changepoints. 
        See \href{https://youtu.be/omOjQgB93Kw}{this url} for a video comparison between \RLPRKF and \RLPRWoLF.
    }
    \label{fig:bocd-lr-stress}
\end{figure}
The constant reaction to outliers in the case of \RLPRKF means that the parameters reset back to the initial prior belief.
As a consequence, the RMSE of \RLPRKF deteriorates. 
On the other hand, \RLPRWoLF  resets less often and accurately adjusts to the regime changes when they do happen. This results in the lowest RMSE among the three methods.

% \subsection{Non-stationary heavy-tailed linear regression -- ablation}
% \label{experiment:heavy-tail-regression-ablation}
% We show further results for the experiment in Section \ref{experiment:heavy-tail-regression}.
% Figure \ref{fig:lr-wolf-rmse-varying-c} shows the RMSE of \RLPRWoLF by varying the choice of soft-threshold $c$.
% \begin{figure}[H]
%     \centering
%     \includegraphics[width=0.5\linewidth]{figures/lr-wolf-rmse-varying-c.png}
%     \caption{
%     RMSE for \RLPRWoLF and \RLPRKF.
%     The horizontal dashed line corresponds to the RMSE under \RLPRKF.
%     The dotted black line corresponds to the RMSE under \RLPRWoLF as a function of the choice of soft-threshold $c$.
%     }
%     \label{fig:lr-wolf-rmse-varying-c}
% \end{figure}
% We observe that choices of $c > 1.5$, \RLPRWoLF outperforms \RLPRKF.
% This is expected because a small value of $c$ means that small deviations are to be considered as outliers.
% The minimum RMSE is obtained with $c\in(4,6)$ and then increases.
% In the limit, when $c\to\infty$, the RMSE of \RLPRWoLF matches that of \RLPRKF.

% Removing for now
\eat{
\subsection{Compute resources}
\label{section:compute-resources}
All experiments were run on a single TPU V2-8 provided by the TPU Research Cloud program.

\begin{table}[htb]
    \centering
    \begin{tabular}{lrr}
        Experiment & running time & comments\\
        \toprule
        % Section \ref{experiment:linear-regression-variable-selection} -- hyperparameter selection & 4min 42secs & hyperparameter selection\\
        % Section \ref{experiment:linear-regression-variable-selection} -- evaluation & 7min 50secs & three runs: one per scenario\\
        Section \ref{experiment:classification} -- hyperparameter selection & 10min 17secs & two runs: one per scenario\\
        Section \ref{experiment:classification} -- evaluation  & 16min 2s & two runs: one per scenario\\
        Section \ref{experiment:heavy-tail-regression} & 1hr 5mins & full-memory models\\
        Figure \ref{fig:lr-wolf-rmse-varying-c} & 22min 14s & 
    \end{tabular}
    \vspace{0.5em}
    \caption{
        Running time for the experiments.
    }
    \label{tab:running-time}
\end{table}

\subsection{Online linear regression with variable selection --- ablation}
\label{experiment:linear-regression-variable-selection-additional}
In this section, we detail the hyperparameter selection and show additional results for the
experiment show in Section \ref{experiment:linear-regression-variable-selection} with
dataset \ref{dataset:lr-variable-selection}.

\paragraph{Hyperparameter selection}
For the methods we study in this experiment,
we design a warmup phase followed by three evaluation phases --- one for each of the three scenarios we outline below.
In the warmup phase, we select the best hyperparameters that minimise the RMSE after a single run of $10,000$ steps
using the Bayesian optimisation library of \cite{nogueira2014BO}.
We detail the search space of the hyperparameters in Table \ref{tab:hparams-lr}.\footnote{The domain of searched hyperparameters can be also found in the file
\texttt{./configs/lr-param-search.toml}.
The resulting hyperparameters can be found in the file \texttt{./configs/lr-param-optim.toml}.}
\begin{table}[H]
    \centering
    \tiny
    \begin{tabular}{lll}
    method & param & search space\\
    \toprule
    \CACI & $\sigma$ & $[0,1]$\\
    \midrule
    
    \CPLCR[-1/-10] & $p(s_t=1)$ & $[0, 1]$\\
    \CPLCR[-1/-10] & $\sigma$ & $[10^{-2}, 1]$\\
    \CPLCR[-1/-10] & $\rho_t$ & $\{1\}$\\
    \midrule
    
    \CPLPR[-1/-10] & $p(s_t=1)$ & $[0, 1]$\\
    \CPLPR[-1/-10] & $\sigma$ & $[10^{-2}, 1]$\\
    \midrule
    
    \CPPACI & l.r. & $[0,1]$ \\
    \CPPACI & $\sigma$ & $[0,2]$ \\
    \CPPACI & i.t. & $\{10\}$\\
    \CPPACI & $(a,b)$ & $\{(1,1\}$\\
    \midrule
    
    \CPPSCR & l.r. & $[0,1]$ \\
    \CPPSCR & $\sigma$ & $[0,2]$ \\
    \CPPSCR & $\rho$ & $\{1\}$ \\
    \CPPSCR & i.t. & $\{10\}$\\
    \CPPSCR & $(a,b)$ & $\{(1,1)\}$\\
    \midrule
    
    \CPPSPR & l.r. & $[0,1]$ \\
    \CPPSPR & $\sigma$ & $[0,2]$ \\
    \CPPSPR & i.t. & $\{10\}$\\
    \CPPSPR & $(a,b)$ & $\{(1,1)\}$\\
    \midrule

    \RLCR[-1/-10] & $p(r_t = i + 1 \vert r_{t-1} = i)$ & $[0,1]$\\
    \RLCR[-1/-10] & $\sigma$ & $[0,1]$\\
    \RLCR[-1/-10] & $\rho$ & $\{1\}$\\
    \midrule

    \RLPR[-1/-10] & $p(r_t = i + 1 \vert r_{t-1} = i)$ & $[0,1]$\\
    \RLPR[-1/-10] & $\sigma$ & $\{1\}$\\
    \midrule

    \RLSPR[-1/-10] & $p(r_t = i + 1\vert r_{t-1} = i)$ & $[0,1]$\\
    \RLSPR[-1/-10] & $\sigma$ & $[10^{-2}, 1.0]$\\
    \midrule

    shared & $\vSigma_0$ & $[0,1]\,\vI$ \\
    \end{tabular}
    \caption{
        Space over searched hyperparameters for the experiment in Section \ref{experiment:linear-regression-variable-selection}.
        Values shown in a range $[a,b]$ for $a < b$ mean that the values were chosen to be within that range.
        Values shown in braces $\{a\}$ mean that the hyparameter was set to value $a$.
        The method `shared' correspond to hyperparameters that were chosen for all hyperparameters.
        The term `l.r.' stands for learning rate.
        The term `i.t.' stands for inner iterations.
        The value $p(r_t = i + 1 | r_{t-1} = i)$ is a constant value for $i \in \{1, \ldots, t\}$.
    }
    \label{tab:hparams-lr}
\end{table}

The configuration of the data-generating process is the following:
the number of features chosen is $k=10$,
the mean-reversion rate of model parameters is $\kappa=0.1$,
the total number of parameters is $m=20$,
the mean-reversion rate is $q_\theta = 0.1$,
and the rate of abrupt changes $p_\epsilon =  0.001$.
After tuning  the hyperparameters, we test each method under three  scenarios:
 a (i) mean-reverting-only scenario, an (ii) abrupt-changes-only scenario, and a (iii) mean-reverting and abrupt-changes scenario.

In experiments (i) and (iii) we set the variance of the true model parameters to be
$q_\theta = 0.1$, and for experiment (ii) we set $q_\theta = 0$ and $\kappa = 0$.
We modulate the mean-reversion with the parameter $\kappa$ and the abrupt changes with $p_\epsilon$.
The (i) mean-reverting-only scenario modifies the DGP by fixing $p_\epsilon = 0$,
so that only one segment is observed;
the (ii) abrupt-changes-only scenario modifies the DGP by fixing $q_\theta = 0$ and $p_\epsilon = 0.005$, 
so that parameters do not mean-revert;
finally, the (iii) mean-reverting and abrupt-changes scenario (both) modify the DGP by fixing
$q_\theta = 0.005$ and $p_\epsilon = 0.005$.

\paragraph{Further results}
Figure \ref{fig:lr-results-over-kf} shows the outperformance of the methods tested in Section \ref{experiment:linear-regression-variable-selection}.
\begin{figure}[htb]
    \centering
    \includegraphics[width=0.8\linewidth]{figures/lr-outperformance-over-kf-all.png}
    \caption{
    Outperformance over \texttt{static} linear model.
    }
    \label{fig:lr-results-over-kf}
\end{figure}
Figure \ref{fig:lr-performance-rmse-all-extend} extends the results shown in Figure \ref{fig:lr-results}
to include \texttt{RLCC} variants.
\begin{figure}[htb]
    \centering
    \includegraphics[width=0.8\linewidth]{figures/lr-performance-rmse-all-extend.png}
    \caption{
    RMSE error for the linear regression with variable selection problem.
    Distribution over $100$ trials.
    }
    \label{fig:lr-performance-rmse-all-extend}
\end{figure}
Figure \ref{fig:sample-run-all-lr} show the RMSE for a single run of the `Both' configuration.
over a \texttt{static} model.
\begin{figure}[htb]
    \centering
    \includegraphics[width=0.8\linewidth]{figures/sample-run-both.png}
    \caption{
    RMSE for a single run of the `Both' configuration for
    the experiment in Section \ref{experiment:linear-regression-variable-selection}.
    }
    \label{fig:sample-run-all-lr}
\end{figure}
}
