# Supplementary material for: A unifying framework for generalised Bayesian online learning in non-stationary environments
Source: arXiv:2411.10153 source file (2025-03-12)
Supplement: Supplementary file 2 [file computing-posteriors.tex]

\section{Choice of posterior computation \cPosterior}
\label{appendix:posterior-computation}
In this section, we provide details about the choices of \cPosterior that estimates the posterior over model parameters one datapoint at a time.

\subsection{Extended Kalman Filter}
Consider the state-space model (SSM)
\begin{equation}\label{eq:EKF-SSM}
\begin{aligned}
    p(\vtheta_t \cond \vtheta_{t-1}) &= {\cal N}(\vtheta_t \cond f_t(\vtheta_{t-1}), \vQ_t),\\
    p(\vy_t \cond \vtheta_t, \vx_t) &= {\cal N}(\vy_t \cond h_t(\vtheta_t, \vx_t), \vR_t),
\end{aligned}
\end{equation}
with
$\vy_t\in\real^\dimobs$ the measurement,
$\vtheta_t \in \real^\dimstate$, the state (model parameters),
$\vx_t \in \real^\dimin$ the exogenous features,
$f_t: \real^\dimstate \to \real^\dimstate$ the state-transition function,
$h_t: \real^{\dimstate}\times\real^\dimin \to \real^\dimobs$ the measurement function, e.g., a neural network,
$\vR_t \in \real^{\dimobs\times\dimobs}$ the measurement covariance, and
$\vQ_t \in \real^{\dimstate\times\dimstate}$ the dynamics covariance.

If both, the measurement function $f_t$ and the state-transition function  $h_t$ 
are differentiable with respect to $\vtheta_t$,
% and the prior distribution over model parameters is
then, the extended Kalman filter (EKF) algorithm provides a recursive formula to approximate the posterior over model parameters
$p(\vtheta_t \cond \data_{1:t})$.

The approximation to $p(\vtheta_t \cond \data_{1:t})$, which we denote 
$q(\vtheta_t \cond \data_{1:t})$, consists of two steps:
the first step predicts the state at time $t$ conditioned on the data up to time $t-1$, i.e.
$q(\vtheta_t \cond \data_{1:t-1})$;
the second steps estimates the approximate posterior $q(\vtheta_t \cond \data_{1:t})$.

\paragraph{The predict step $q(\vtheta_t \cond \data_{1:t-1})$.}
Let $t \geq 1$ and $q(\vtheta_{t-1} \cond \data_{1:t-1}) = {\cal N}(\vtheta_{t-1} \cond \vmu_{t-1}, \vSigma_{t-1})$
with $\vmu_{t-1}$ the approximate posterior mean and $\vSigma_{t-1}$ the approximate posterior covariance.
The predict step replaces $f_t$ in \eqref{eq:EKF-SSM} with a first order approximation of $f_t$
around the previous mean $\vmu_{t-1}$. Let
\begin{equation}
    \bar{f}_t(\vtheta_t) = f_t(\vmu_{t-1}) + \vF_t(\vtheta_t - \vmu_{t-1}),
\end{equation}
be the approximate transition function with
$\vF_t$ the Jacobian of $f_t$ evaluated at $\vmu_{t-1}$.
Then, the predict step takes the form
\begin{equation}\label{eq:ekf-predict}
\begin{aligned}
    q(\vtheta_t \cond \data_{1:t-1})
    &= \int q(\vtheta_t, \vtheta_{t-1} \cond \data_{1:t-1}) \d\vtheta_{t-1}\\
    &= \int {\cal N}(\vtheta_t \cond \bar{f}_t(\vtheta_{t-1}), \vQ_t)\, q(\vtheta_{t-1} \cond \vtheta_{t-1}) \d\vtheta_{t-1}\\
    &= \int {\cal N}(\vtheta_t \cond \bar{f}_t(\vtheta_{t-1}), \vQ_t)\, {\cal N}(\vtheta_{t-1} \cond \vmu_{t-1}, \vSigma_{t-1}) \d\vtheta_{t-1}\\
    &= {\cal N}(\vtheta_t \cond \vmu_{t | t-1}, \vSigma_{t | t-1})
\end{aligned}
\end{equation}
with
\begin{align}
    \vSigma_{t | t-1} &= \vF_t\,\vSigma_{t-1}\,\vF_{t}^\intercal + \vQ_t,\\
    \vmu_{t | t-1} &= \vF_t\,\vmu_{t-1}.
\end{align}

\paragraph{The update step $q(\vtheta_t \cond \data_{1:t})$.}
Let $t \geq 1$ and $q(\vtheta_t \cond \data_{1:t-1}) = {\cal N}(\vtheta_t \cond \vmu_{t|t-1}, \vSigma_{t|-1})$
given by \eqref{eq:ekf-predict}.
The update step replaces $h_t$ in \eqref{eq:EKF-SSM} with a first order approximation of $h_t$ around
the previous predicted mean $\vmu_{t|t-1}$.
Let
\begin{equation}
    \bar{h}_t(\vtheta_t, \vx_t) = h_t(\vmu_{t-1}, \vx_t) + \vH_t\,(\vtheta_t - \vmu_{t-1}),
\end{equation}
be the approximate measurement function with
$\vH_t$ the Jacobian of $h_t$ under $\vtheta$ evaluated at $(\vmu_{t|t-1}, \vx_t)$.
The update step takes the form
\begin{equation}
\begin{aligned}
    q(\vtheta_t \cond \data_{1:t})
    &\propto {\cal N}(\vy \cond \bar{h}_t(\vtheta_t, \vx_t), \vR_t)\,q(\vtheta_t \cond \data_{1:t-1})\\
    &\propto {\cal N}(\vy \cond \bar{h}_t(\vtheta_t, \vx_t), \vR_t)\,{\cal N}(\vtheta_t \cond \vmu_{t|t-1}, \vSigma_{t|t-1})\\
    &\propto {\cal N}(\vtheta_t \cond \vmu_t, \vSigma_t),
\end{aligned}
\end{equation}
with
\begin{equation}\label{eq:ekf-predict-step}
\begin{aligned}
    \hat{\vy}_t &= h_t(\vmu_{t|t-1}, \vx_t)\\
    \vS_t &= \vH_t\,\vSigma_{t|t-1}\,\vH_t^\intercal + \vR_t,\\
    \vK_t &= \vSigma_{t|t-1}\,\vH_t^\intercal\,\vS_t^{-1},\\
    \vmu_t &= \vmu_{t|t-1} + \vK_t(\vy_t - \hat{\vy}_t),\\
    \vSigma_t &= \vSigma_{t|t-1} - \vK_t\,\vS_t\,\vK_t^\intercal.
\end{aligned}
\end{equation}

\subsection{Kalman filter}
The Kalman filter (KF) is a special case of the EKF where the state-transition and measurement functions are linear, i.e.,
\begin{equation}\label{eq:kf-measurement}
\begin{aligned}
    p(\vtheta_t | \vtheta_{t-1}) &= {\cal N}(\vtheta_t \cond \vF_t\,\vtheta_{t-1}, \vQ_t),\\
    p(\vy_t \cond \vtheta_t) &= {\cal N}(\vy_t \cond \vH_t\,\vtheta_t, \vR_t).
\end{aligned}
\end{equation}

\subsection{Exponential-family extended Kalman filter}
Closed-form updates are available when the measurement model is a member of the exponential family. This is due to the work of \cite{olllivier2018expfamekf}, which we briefly summarise here. 

Suppose that our measurement model is of the form
\begin{equation}\label{eq:expfam-measurement}
p(\vy_t | \vtheta_t) = \frac{1}{Z(\veta_t)}\exp\Big(\veta_t^\intercal T(\vy_t) + b(\vy_t) \Big)
\end{equation}
where $\veta_t = h_t(\vtheta_t)$ are the natural parameters, 
$T$ is the sufficient statistic,
and $Z(\veta_t)$ is the log-partition function.
For brevity, we will write $\vz_t = T(\vy_t)$.
The ExpfamEKF replaces the mean $\hat{\vy_t}$ and measurement covariance $\vR_t$ in the predict step \eqref{eq:ekf-predict-step}
with
\begin{equation}
\begin{aligned}
    \hat{\vy_t} &= \frac{\partial}{\partial\veta_t}Z(\veta_t),\\
    \vR_t &= \frac{\partial^2}{\partial\veta_t^2} Z(\veta_t).
\end{aligned}
\end{equation}

\subsection{Weighted-observation likelihood filter}
The EKF variaiant of the weighted-observation likelihood filter (WoLF) of \cite{duranmartin2024-wlf}
proposes a robust version of the EKF in the presence of outliers and misspecified measurement models.
Their method modifies the measurement covariance $\vR_t$ in the EKF predict step \eqref{eq:ekf-predict-step}
with
\begin{equation}
    \hat{\vR}_t = \vR_t/ W_t(\vy_t,\hat{\vy}_t)^2.
\end{equation}
Here, $W_t(\vy_t, \hat{\vy}_t)$ is the weighting function. In this paper, we consider the IMQ weighting function
\begin{equation}
    W(\vy_t, \hat{\vy}_t) = \left(1 + \frac{\|\vy_t - \hat{\vy}_t\|^2}{c^2}\right),
\end{equation}
with $c > 0$.
