# Supplementary material for: A unifying framework for generalised Bayesian online learning in non-stationary environments
Source: arXiv:2411.10153 source file (2025-03-12)
Supplement: Supplementary file 3 [file datasets-explain.tex]

\section{Datasets}

% Removing for now
\eat{
\subsection{Online linear regression with variable selection --- dataset specification}
\label{dataset:lr-variable-selection}
In this experiment, we consider a stream of data-points whose data-generating process (DGP) 
has a slowly-changing component and an abruptly-changing component.
The slowly-drifting component is characterised by a mean-reverting process over the true (unobserved) model parameters $\vtheta$. More precisely, 
\begin{align}
\vtheta_t &= \vtheta_{t-1} + \kappa\,({\bf 1}_m - \vtheta_{t-1}) + \vepsilon_t\,,
\end{align}
where $\kappa>0$ is the mean-reversion rate of model parameters $\vtheta_t\in\mathbb{R}^\dimstate$ towards ${\bf 1}_m =(1, \ldots, 1) $, 
$\vepsilon_t$ is an $\dimstate$-dimensional Gaussian with covariance $q_\theta\,\vI$ and zero mean, and we take $\vtheta_0 =  {\bf 1}_m$ and $q_\theta>0$.
The observation $y_t\in\real$ is given by 
\begin{align}
     y_t  &\sim {\cal N}(\varphi_t^\intercal\,\vtheta_t, 1)\,,
\end{align}
where $\varphi_t\in\real^\dimstate$ encodes the non-stationarity in the observations. 
We call $\varphi_t$ the active parameters and we take them to be modulated by a abruptly-changing process $\vm$ that selects the features used to produce an observation.
More precisely, 
\begin{align*}
\varphi_t &= \vm_t \odot \phi(x_t)\,,&
\vm_t &=
    \begin{cases}
      \vm_{t-1}  & \text{if } c_t = 0\,,\\
     {\rm M}(m, k) & \text{if } c_t = 1,
    \end{cases}&
{c_t} &=
    \begin{cases}
        0 & \text{w.p. } 1 - p_\epsilon\,,\\
        1 & \text{w.p. } p_\epsilon\,,
    \end{cases}&
    x_t &\sim {\cal U}[-3, 3]\,,    
\end{align*}
%where ${\rm MHyp}(\dimstate, k)$ is a sample from an $\dimstate$-dimensional multivariate Hypergeometric distribution with $k$ draws,
where $0<p_\epsilon\ll 1$ is the probability of a changepoint,  ${\rm M}(\dimstate, k)$ is a sample from an $\dimstate$-dimensional multivariate distribution in $\{0,1\}^\dimstate$ such that the sum of entries is always $k$ and each possibility has probability $k!\,(\dimstate-k)!/\dimstate!$, and
${\cal U}[a, b]$ is a uniform random variable between $a$ and $b$.
The map $\phi:\mathbb{R}\to\mathbb{R}^\dimstate$ is designed to encode various frequencies and is defined by
\begin{equation}
    \phi(x) = 
    \begin{bmatrix}
    1, & x, & \cos(x), & \sin(\pi d_1), & \ldots, & \sin(\pi d_{\dimstate-3})
    \end{bmatrix},
\end{equation}
with $d_i = f_\text{start} + i\,\Delta$, $i = 0, \ldots, \dimstate$, and $\Delta = (f_\text{stop} - f_\text{start}) / (k - 3 - 1)$.
In summary, at each step a measurement is produced by $k$ of the $m$ features.
The $k$ chosen features remain the same until there is a change, that is,  whenever $c_t = 1$. The frequency with which these abrupt changes occur is modelled through the parameter $p_\epsilon$.

Figure \ref{fig:segments-lr} show a sample run of the experiment in Section \ref{experiment:linear-regression-variable-selection}.
\begin{figure}[H]
    \centering
    \includegraphics[width=0.45\linewidth]{figures/lr-params-sample.png}
    \includegraphics[width=0.45\linewidth]{figures/segments-lr.png}
    \caption{    
    We show six regimes (labelled S0, S1, S2, S3, S4, and S5 in the plots).
    Each regime is characterised by the four parameters (out of a total of ten parameters) that are used to produce measurements.
    A regime change happens, at a given timestep, with probability $p_\epsilon=0.005$.
    The \textbf{left panel} shows the evolution of the active parameters, that is, the parameters that will be used to produce measurements.
    In each segment, we show the trajectory of the four parameters that are used to produce the measurements. However, in the background, all parameters
    evolve according to the mean-reverting process.
    The \textbf{right panel} shows the measurements over the six regimes shown in the left panel.
    The grey dots represent the measurements and the black lines represent the mean of the measurement process.
    }
    \label{fig:segments-lr}
\end{figure}
}

\subsection{Modified 1d-MNIST dataset}
\label{appendix:dataset-modified-1d-mnist}
This dataset is a modification of the 1D-MNIST dataset in \cite{greydanus20201dmnist}.
We consider the ``platonic'' base classes shown in Figure \ref{fig:1d-mnist-platonic}.
\begin{figure}[H]
    \centering
    \includegraphics[width=1.0\linewidth]{figures/1dmnist-base.png}
    \caption{
        Platonic figures for the 1D-MNIST dataset.
    }
    \label{fig:1d-mnist-platonic}
\end{figure}
To create an instance of each class, we consider the following transformations of an initial vector $\vx\in\real^{12}$ of values representing one of the platonic classes above:
\begin{enumerate}[label=(\roman*)]
    \item padding: this transformation adds zeros to the right of the vector of values. The size of the pad is drawn from a
    discrete uniform ${\cal U}\{p_{\rm min}, p_{\rm max}\}$ with $p_{\rm min} < p_{\rm max}$.\footnote{Here, we use $\{\cdot,\,\cdot\}$ in  $U\{a,b\}$ to denote a discrete uniform random variable on the integers between $a$ and $b$.}
    \item contraction: shrinks the resulting vector into $\real^{\ell_c}$ using linear interpolation.
    \item scale: multiplies the values in the vector by the scalar $(1 + u_s)$, with $u_s \sim {\cal N}(-0.5, \sigma_s^2)$
    \item translate: circular shift the elements of the vector  $u_t$ units to the right, with $u_t \sim {\cal U}\{0, m_t\}$.
    \item correlated noise: samples a total of $\ell_c$ Gaussian random variables with zero mean
    and scale $\rho_s$. These random variables are then passed through a Gaussian filter (convolution)
    with standard deviation of $2$. The resulting noise is added to the vector.
    \item i.i.d. noise: samples from a multivariate Gaussian ${\cal N}({\bm 0}, i_s^2{\bf I})$
    and adds its value to the vector. Here, $i_s>0$ is the scale parameter of the i.i.d.~noise.
    \item resize: specifies the final size of the vector to be $\ell_f$
\end{enumerate}

We provide an example. Let $\vx = (x_1,\dots,x_{12})$, and assume we sample the value $p\in\{p_{\rm min},\dots,p_{\rm max}\}$. Then, after padding, the resulting vector is $$(x_1,\dots,x_{12},\underbrace{0,\dots,0}_{\text{$p$ times}})\,.$$  
Next, the contraction takes the values $(i/(12+p),\,x_i)_{i=1}^{12+p}$ where $x_i=0$ for $i>12$ and obtains, using linear interpolation, values for the $y_i$'s in the vector $(i/\ell_c,\,  y_i)_{i=1}^{\ell_c}$. The resulting vector $\bm{y}=(y_1,\dots, y_{\ell_c})$ is scaled to obtain $(1+u_s)\,\bm{y}$. For a circular shift sample $u\in\{0,\dots,m_t\}$, the vector $\bm{y}$ becomes
\begin{equation}
\bm{y} =    \left(y_{1+u \text{ mod } \ell_c},\dots, y_{\ell_c + u \text{ mod } \ell_c}\right)\,.
\end{equation}
Then, for the correlated noise, we follow (v) to create the vector $\bm{z}_1\in\real^{\ell_c}$ and $\bm{y}$ transforms to $\bm{y}+\bm{z}_1$. Similarly, we create a vector of i.i.d.~noise $\bm{z}_2$ and update $\bm{y}$ to be $\bm{y}+\bm{z}_2$. Lastly, we perform a linear interpolation as before to obtain a final vector in $\real^{\ell_f}$.

Table \ref{tab:1dmnist-params} shows the values that we use for the hyperparameters above.

\begin{table}[H]
    \centering
    \begin{tabular}{ccc}
        variable & name in the code & default value\\
        \toprule
        $\ell_c$ & \texttt{template\_len} & $12$\\
        $[p_\text{min}, p_\text{max}]$ & \texttt{padding} & $[0,40]$\\
        $\sigma_s$ & \texttt{scale\_coeff} & $0.0$\\
        $m_t$ & \texttt{max\_translation} & 40\\
        $\rho_s$ & \texttt{corr\_noise\_scale} & 0.0\\
        $i_s$ & \texttt{iid\_noise\_scale} & $5\times10^{-2}$\\
        $\ell_f$ & \texttt{final\_seq\_length} & 50\\
         &  & \\
    \end{tabular}
    \caption{
        Default parameters for the 1D-MNIST.
    }
    \label{tab:1dmnist-params}
\end{table}

\subsubsection{Non-stationary correlated noise}
\label{dataset:1d-mnist-correlated-noise}
In this experiment, we consider the five first platonic classes of the 1D-MNIST dataset.
We create modified instances of each class adjusted by the transformations outlined above.
At every timestep, with probability $p_\epsilon > 0$,
we sample the `\texttt{scale}' value from a 
${\rm Beta}(2,5)$.
See Figure \ref{fig:1d-mnist-scale} for samples of the
`0'-class with padding, interpolation, translation, and correlated noise.
Each panel corresponds to a sample different levels of \texttt{scale}.
\begin{figure}[H]
    \centering
    \includegraphics[width=1\linewidth]{figures/1dmnist-corr.png}
    \caption{
        Instance of transformed class-0 with padding, random translation, and no i.i.d. noise.
        Different regimes correspond to different correlated noise scales.
        The orange line corresponds to the underlying \textit{platonic} representation of the class,
        the blue line corresponds to the correlated noise.
        The observed representation is show in the black dotted line.
    }
    \label{fig:1d-mnist-scale}
\end{figure}

\subsubsection{Label permutation}
\label{dataset:1d-mnist-label-permutation}
In this experiment %, we consider a fixed set of hyperparameters used to generate new classes.
we sample  5 randomly-chosen classes without replacement, which we label from $0$ to $4$.
At each timestep, with probability $p_\epsilon$, we sample another set of 5-randomly chosen
classes which we then label from $0$ to $4$.
% This dataset is the 1D-MNIST equivalent to the split-MNIST dataset typically considered in CL papers \gdm{CITECITECITE}.

Figure \ref{fig:1d-mnist-base-sample} shows an illustrative sample of
the non-stationary correlated noise configuration in Subsection \ref{dataset:1d-mnist-correlated-noise}, and
the label permutation configuration in Subsection \ref{dataset:1d-mnist-label-permutation}.
\begin{figure}[H]
    \centering
    \includegraphics[width=1.0\linewidth]{figures/1dmnist-noise-sample.png}
    \includegraphics[width=1.0\linewidth]{figures/1dmnist-class-sample.png}
    \vspace{-2em}
    \caption{
    Illustrative examples of the transformations of the 1D-MNIST dataset.
    The \textbf{top panel} shows a sample from the correlated noise experiment.
            The title shows the level of noise in each simulation.
    The \textbf{bottom panel} shows a sample from the label permutations experiment.
            The title shows the label assigned to the platonic class 0.
    Each column in the figure represents a regime.
    }
    \label{fig:1d-mnist-base-sample}
\end{figure}
