# Supplementary material for: A unifying framework for generalised Bayesian online learning in non-stationary environments
Source: arXiv:2411.10153 source file (2025-03-12)
Supplement: Supplementary file 4 [file source-code-example.tex]

\section{Source code}
\label{appendix:source-code}

\paragraph{Linear regression with known variance via \RLPR}
The snippet below shows how to fit a linear-regression model with known variance.
The measurement model takes the form $h_t(\vtheta_t) = \vtheta_t^\intercal\vx_t$.

\begin{lstlisting}[escapechar=\%, frame=single]
import jax.numpy as jnp
from %\abonelib%.methods.gauss_filter import GaussianFilter
from %\abonelib%.methods.adaptive import ExpfamRLPR

def apply_fn(theta, x):
    return jnp.atleat_1d(theta @ x)

# Load filters
K = 10 # number of trajectories
p_change = 0.01 # constant hazard rate
base_filter = GaussianFilter(
    apply_fn, dynamics_covariance=0.0, variance=1.0
)
bocd_filter = ExpfamRLPR(p_change, K, base_filter, method="prior-reset")

# filter
bel = bocd_filter.init_bel(wprior, wcov_prior, 0.0)
bel, hist_bocd = bocd_filter.scan(y[:, None], X, bel, callback)
\end{lstlisting}

\paragraph{Classification neural network via \RLSPR}
Next, we show how to fit a two-layered neural network with 50 units each.
We note that the only two changes from the code above are the measurement model
specification and \cPosterior, which is now given by \texttt{MultinomialFilter}.

\begin{lstlisting}[escapechar=\%, frame=single]
import flax.linen as nn
import jax.numpy as jnp
from %\abonelib%.methods.gauss_filter import MultinomialFilter
from %\abonelib%.methods.adaptive import ExpfamRLSPR

class NNet(nn.Module):
    n_units: int = 50
    @nn.compact
    def __apply__(self, x):
        x = nn.Dense(self.n_units)(x)
        x = nn.relu(x)
        x = nn.Dense(self.n_units)(x)
        x = nn.relux(x)
        return x

model = NNet()

# Load filters
K = 10 # number of hypotheses
p_change = 0.01 # constant hazard rate
base_filter = MultinomialFilter(
    model.apply, dynamics_covariance=0.0, variance=1.0
)
adaptive_filter = ExpfamRLSPR(p_change, K, base_filter)

# filter
bel = adaptive_filter.init_bel(wprior, wcov_prior, 0.0)
bel, hist_filter = adaptive_filter.scan(y[:, None], X, bel, callback)
\end{lstlisting}
