# Supplementary material for: A unifying framework for generalised Bayesian online learning in non-stationary environments
Source: arXiv:2411.10153 source file (2025-03-12)
Supplement: Supplementary file 5 [file computing-conditional-priors.tex]

\section{Choice of conditional prior \cPrior}
\label{appendix:prior-computation}
In this section, we provide choices of $\gamma_t$ and $\rho_t$ introduced in Section \ref{sec:conditional-prior}.
%as a function of their auxiliary variable $\auxv_t$ that we study in this paper.

\subsection{Runlength \texttt{RL}}
%We take $\auxv_t = r_t$ be the number of timesteps since the last changepoint.
For the choice \texttt{SPR},
we take $\gamma_t = \nu_t(r_t)$ if $r_t>0$ and $\gamma_t = 1$ if $r_t=0$;
the choice \texttt{PR} considers
$\gamma_t = {\mathds 1}(r_t = 0)$.
The choice \texttt{CR}, considers $\gamma_t = \mathds{1}(r_t = 0)$ and $\rho_t = \rho \in (0,1]$ a fixed value.

\subsection{Changepoint location \texttt{CPL}}
%We take $\auxv_t = s_{1:t}$ be the location of changepoints.
For the choices \texttt{PR} and \texttt{CR}, we take $\gamma_t = \mathds{1}(s_t = 1)$
with $\rho_t=\rho\in (0,1]$ a constant value.

\subsection{Changepoint probability \texttt{CPP}}
The choices \texttt{SPR}, \texttt{SCR}, and \texttt{ACI} take $\gamma_t = \upsilon_t$ where $\upsilon_t$ is the changepoint probability (auxiliary variable).

\subsection{Constant \texttt{C}}
The constant (dummy) auxiliary variable takes $\auxv = 0$.
The auxiliary process $\auxv$ affects the prior predictive in a constant manner.
The choice \texttt{ACI} takes $\gamma_t = \gamma \in [0, 1]$ to be a constant value.
